# Supplementary material for: Spin-flip Bethe-Salpeter equation approach for ground and excited states of open-shell molecules and defects in solids
Source: arXiv:2207.04549 ancillary file (2022-07-10)
Supplement: Supplementary file 1 [file SI.pdf]

# Supporting Information: Spin-flip Bethe-Salpeter equation approach for ground and excited states of open-shell molecules and defects in solids

Bradford A. Barker* and David A. Strubbe*

*Department of Physics, University of California, Merced, CA 95343, USA*

E-mail: bbarker6@ucmerced.edu; dstrubbe@ucmerced.edu

# 1 Computational parameters

We use Optimized Norm-Conserving Vanderbilt pseudopotentials[S1] from the Pseudo-Dojo pseudopotential database.[S2]

For ethylene, the relaxed atomic coordinates (at 0°) were calculated with a 0.115 Å real-space grid spacing, equivalent to roughly 115 Ry planewave wavefunction cutoff, in a box with edge-length 12 Å. A smaller box size was used in the subsequent calculations, which contains 99% of the charge density for both the ethylene molecule with no torsion and 90° of torsion.

The ground- and excited-state energies were calculated explicitly at torsions of 0, 5, 10, 15, 30, 45, 60, 75, 80, 85, and 90°. For DFT input to SF-BSE calculations, we used a real-space grid spacing for both the wavefunctions and density of 0.34 Bohr, equivalent to about 85 Ry planewave cutoff for the wavefunctions. Based on van Setten et al.[S3], we used 860 empty states and 24 Ry for the calculation of the screened Coulomb interaction. The SF-BSE Hamiltonian was constructed with 5 occupied orbitals (the maximum number common to both spin channels) and 55 unoccupied orbitals.

For $NV^-$, the localization of the defect wavefunction allows us to use a 2×2×2 supercell (63 atoms) for these calculations, based on just the Γ point (Fig. S8). The dielectric matrix is calculated with 300 empty states and a cutoff of 12 Ry.[S4] The SF-BSE Hamiltonian is constructed from 12 occupied and 11 unoccupied orbitals.

# 2 Method of computing $\langle \hat{S}^2 \rangle$ for spin-flip transitions

As shown in Fig. S1: suppose we have a spin-polarized system with $N = N_\alpha + N_\beta$ electrons such that $N_\alpha > N_\beta$. The high-spin reference state from DFT gives us a set of $\alpha$-spin KS orbitals $\phi_m$ and $\beta$-spin orbitals $\psi_n$, with $m \in \{1, \dots, N_\alpha\}$ and $n \in \{1, \dots, N_\beta, N_\beta + 1, \dots, N_\beta + N_{\mathrm{unocc}}\}$. The orbitals $n \in \{1, \dots, N_\beta\}$ are always occupied; for the state $|N, I\rangle$, one of the orbitals $i \in \{1, \dots, N_\alpha\}$ becomes unoccupied (counting down: $N_\alpha + 1 - i$) while

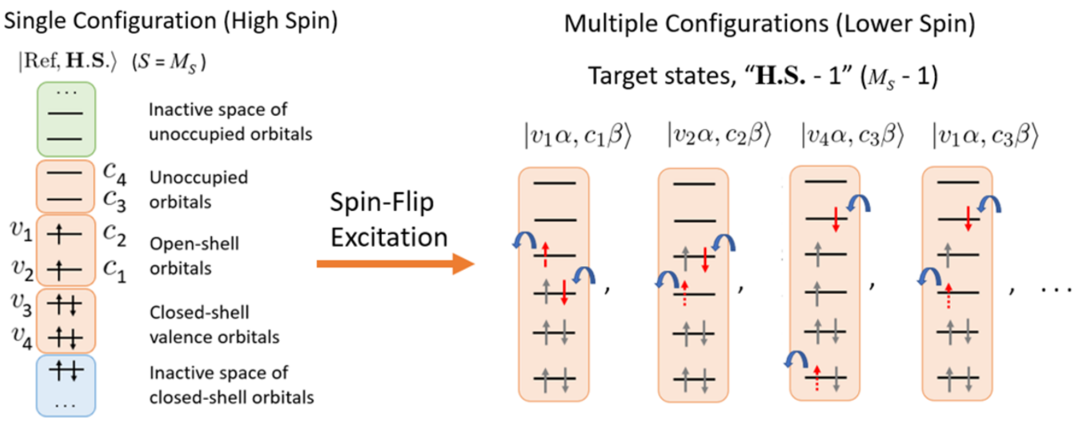


Figure S1: Schematic of the spin-flip method. For SF-BSE, the spin-flip excitation is calculated via the Bethe-Salpeter equation.

one of the orbitals $j \in \{N_\beta + 1, \ldots, N_\beta + N_{\text{unocc}}\}$ becomes occupied (counting up: $N_\beta + j$).

$\langle \hat{S}^2 \rangle_0$ for the ground state (or high-spin reference state) can be readily computed from the well-known Löwdin Formula:[S5]

$$\langle N, 0|\hat{S}^2|N, 0\rangle = \left(\frac{n_\uparrow - n_\downarrow}{2}\right)\left(\frac{n_\uparrow - n_\downarrow}{2} + 1\right) - \sum_{i,\bar{j}} |\langle i|\bar{j}\rangle|^2, \tag{1}$$

where $|N, 0\rangle$ is the ground state or reference state many-body wavefunction. In Fig. S2, we see that $\langle \hat{S}^2 \rangle_0$ deviates very little from 2.0 for all angles, as expected for the triplet spin symmetry of the high-spin reference state. Likewise, $\langle \hat{S}^2 \rangle_0$ for the triplet ground state of the $NV^-$ center is 2.05.

For excitations of the ground state or the high-spin reference state within SF-BSE, we compute the difference between $\langle \hat{S}^2 \rangle$ for the $I$'th spin-flipped excitation and the reference state, 0. This difference is $\Delta\langle \hat{S}^2 \rangle_I$, and the sum of this with $\langle \hat{S}^2 \rangle_0$ gives $\langle \hat{S}^2 \rangle_I$. While the formula for $\Delta\langle \hat{S}^2 \rangle_I$ in the context of SF-TDDFT was previously published as Eq. A10 in Li et al.[S6], was evidently implemented in codes for use in calculations such as Xu et al.[S7], and was used for SF-BSE in Monino and Loos[S8], we work through the formula here as it has remained obscure in the literature. Since the eigenvectors of the Bethe-Salpeter Equation are the electron-hole amplitudes[S9] that are required to construct the two-particle reduced

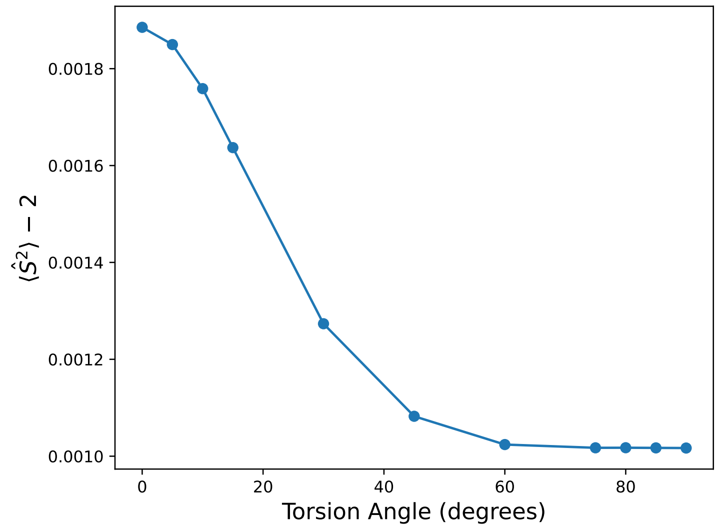


Figure S2: The computed value of $\langle \hat{S}^2 \rangle - 2$ for the (triplet) ethylene high-spin reference state as a function of torsion angle.

difference density matrix $\Delta\Gamma$, we use the formalism developed in Ipatov et al.[S10], originally for spin-conserving transitions and obtained from considering TD Hartree-Fock, and apply it to spin-flipping transitions. With this formalism, we evaluate the $I$'th excited-state $\langle \hat{S}^2 \rangle_I$ by computing first the ground state (or high-spin reference state) $\langle \hat{S}^2 \rangle_0$ from the well-known Löwdin Formula:[S5]

$$\langle \Psi^{\text{H.S. Ref}} | \hat{S}^2 | \Psi^{\text{H.S. Ref}} \rangle = \left( \frac{n_\uparrow - n_\downarrow}{2} \right) \left( \frac{n_\uparrow - n_\downarrow}{2} + 1 \right) - \sum_{i,\bar{j}} |\langle i | \bar{j} \rangle|^2 \tag{2}$$

and then $\Delta\langle \hat{S}^2 \rangle_I$ from a "super-operator" approach:

$$\Delta\langle \hat{S}^2 \rangle_I = \langle \hat{S}^2 \rangle_I - \langle \hat{S}^2 \rangle_0 = \sum_{r,s,\bar{p},\bar{q}} \Delta\Gamma_{r\uparrow,\bar{q}\downarrow,\bar{p}\downarrow,s\uparrow} \langle s|\bar{q}\rangle \langle \bar{p}|r\rangle \,, \tag{3}$$

$$\Delta\Gamma_{r\uparrow,\bar{q}\downarrow,\bar{p}\downarrow,s\uparrow} = \sum_{i\uparrow,\bar{a}\downarrow,j\uparrow,\bar{b}\downarrow} \left( A^I_{i\uparrow,\bar{a}\downarrow} \right)^* A^I_{j\uparrow,\bar{b}\downarrow} \langle N,0| \left[ i^\dagger_\uparrow \bar{a}_\downarrow \,, \left[ \bar{p}^\dagger_\downarrow s^\dagger_\uparrow \bar{q}_\downarrow r_\uparrow \,, \bar{b}^\dagger_\downarrow j_\uparrow \right] \right] |N,0\rangle \,. \tag{4}$$

Here, we use the convention from the quantum chemistry literature that $i$, $j$, $k$ are indexes for creation/annihilation operators for occupied orbitals or bands; $a$, $b$, unoccupied orbitals or bands; and $p$, $q$, $r$, and $s$, either occupied or unoccupied. The use of the over-bar allows

for unrestricted orbitals or, equivalently, spin-polarized bands.

The evaluation of the matrix elements are assisted by the use of the SNEG[S11] software capable of symbolic evaluation of second-quantization-operator expressions. As in Wang et al.[S12], we explicitly consider four cases: (1) $i = j$, $\bar{a} = \bar{b}$, (2) $i \neq j$, $\bar{a} = \bar{b}$, (3) $i = j$, $\bar{a} \neq \bar{b}$, (4) $i \neq j$, $\bar{a} \neq \bar{b}$:

$$\begin{aligned}
&\langle N,0| \left[ i_\uparrow^\dagger \bar{a}_\downarrow \, , \, \left[ \bar{p}_\downarrow^\dagger s_\uparrow^\dagger \bar{q}_\downarrow r_\uparrow \, , \, \bar{b}_\downarrow^\dagger j_\uparrow \right] \right] |N,0\rangle \\
&= \langle N,0| i_\uparrow^\dagger \bar{a}_\downarrow \bar{p}_\downarrow^\dagger s_\uparrow^\dagger \bar{q}_\downarrow r_\uparrow \bar{b}_\downarrow^\dagger j_\uparrow |N,0\rangle - \langle N,0| i_\uparrow^\dagger \bar{a}_\downarrow \bar{b}_\downarrow^\dagger j_\uparrow \bar{p}_\downarrow^\dagger s_\uparrow^\dagger \bar{q}_\downarrow r_\uparrow |N,0\rangle,
\end{aligned} \tag{5}$$

after recognizing that terms with $\bar{a}_\downarrow |N,0\rangle = 0$. Similarly, terms with $\langle N,0|\bar{b}_\downarrow^\dagger = 0$, reducing the number of non-trivial terms in Eq. 5. Finally, we recognize that terms such as $\langle N,0| i_\uparrow^\dagger \bar{p}_\downarrow^\dagger s_\uparrow^\dagger \bar{q}_\downarrow r_\uparrow i_\uparrow |N,0\rangle$ can be considered as $\left(\langle N,0| i_\uparrow^\dagger\right) \bar{p}_\downarrow^\dagger s_\uparrow^\dagger \bar{q}_\downarrow r_\uparrow \left(i_\uparrow |N,0\rangle\right)$; that is, the matrix element is taken with respect to a high-spin reference state many-body wavefunction in which the electron in the $i_\uparrow$ orbital has been removed.

We consider explicitly the matrix element in the contribution to $\Delta\Gamma_{r\uparrow,\bar{q}\downarrow,\bar{p}\downarrow,s\uparrow}$ for the case when $i = j$ and $a = b$:

$$\begin{aligned}
&\langle N,0| i_\uparrow^\dagger \bar{a}_\downarrow \bar{p}_\downarrow^\dagger s_\uparrow^\dagger \bar{q}_\downarrow r_\uparrow \bar{b}_\downarrow^\dagger j_\uparrow |N,0\rangle - \langle N,0| i_\uparrow^\dagger \bar{a}_\downarrow \bar{b}_\downarrow^\dagger j_\uparrow \bar{p}_\downarrow^\dagger s_\uparrow^\dagger \bar{q}_\downarrow r_\uparrow |N,0\rangle \\
&= \langle N,0| \delta(\bar{a},\bar{a}) i_\uparrow^\dagger \bar{p}_\downarrow^\dagger s_\uparrow^\dagger \bar{q}_\downarrow r_\uparrow i_\uparrow |N,0\rangle - \langle N,0| \delta(\bar{a},\bar{p}) \delta(\bar{a},\bar{q}) i_\uparrow^\dagger s_\uparrow^\dagger r_\uparrow i_\uparrow |N,0\rangle \\
&- \langle N,0| \delta(\bar{a},\bar{a}) i_\uparrow^\dagger \bar{p}_\downarrow^\dagger s_\uparrow^\dagger \bar{q}_\downarrow r_\uparrow i_\uparrow |N,0\rangle + \langle N,0| \delta(\bar{a},\bar{a}) \delta(i,s) i_\uparrow^\dagger \bar{p}_\downarrow^\dagger \bar{q}_\downarrow r_\uparrow |N,0\rangle.
\end{aligned} \tag{6}$$

The first and third terms cancel, giving the contribution

$$\Delta\Gamma_{r\uparrow,\bar{q}\downarrow,\bar{p}\downarrow,s\uparrow}(i=j, a=b \text{ only}) = \sum_{i\uparrow,\bar{a}\downarrow} \left(A^I_{i\uparrow,\bar{a}\downarrow}\right)^* A^I_{i\uparrow,\bar{a}\downarrow} \left( \sum_k |\langle k|\bar{a}\rangle|^2 - \sum_{\bar{k}} |\langle i|\bar{k}\rangle|^2 - |\langle i|\bar{a}\rangle|^2 \right), \tag{7}$$

with the convention that $k$ and $\bar{k}$ are occupied states from the ground state or high-spin reference state.

After straightforward but tedious algebra to arrive at the contributions from the remaining cases, we arrive at the expressions below:

$$\begin{aligned}\Delta\langle\hat{S}^2\rangle_I =& 1 - 2M_S^{\text{H.S. Ref}} + \sum_{i,\bar{a},j,\bar{b}} \\ & \Bigg\{ \left(A^I_{j\uparrow,\bar{b}\downarrow}\right)^* A^I_{i\uparrow,\bar{a}\downarrow} - \delta_{i,j}\delta_{\bar{a},\bar{b}} \left(\sum_k |\langle k|\bar{a}\rangle|^2 - \sum_{\bar{k}} |\langle i|\bar{k}\rangle|^2 - |\langle i|\bar{a}\rangle|^2\right) \\ & + (1-\delta_{i,j})\delta_{\bar{a},\bar{b}} \sum_{\bar{k}} \langle j|\bar{k}\rangle\langle\bar{k}|i\rangle - \delta_{i,j}(1-\delta_{\bar{a},\bar{b}}) \sum_k \langle k|\bar{b}\rangle\langle\bar{a}|k\rangle - \langle i|\bar{b}\rangle\langle\bar{a}|i\rangle \\ & + (1-\delta_{i,j})(1-\delta_{\bar{a},\bar{b}})\langle j|\bar{b}\rangle\langle\bar{a}|i\rangle \Bigg\}, \end{aligned} \tag{8}$$

where $k$ is the index for the $k$'th occupied up-spin orbital in the high-spin reference state, and $\bar{k}$, down-spin. This equation has an important property of gauge-invariance which can be explicitly verified: a phase change of an individual orbital, or orbital rotation within a degenerate subspace, does not affect the final result, provided that the coefficients $A$ have the counteracting change that keeps the quasiparticle wavefunction $\Psi^I$ constant. For ease of implementation, we add and subtract terms involving the unoccupied $i$ orbital to include this orbital in sums over $k$. The constant term $1 - 2M_S^{\text{H.S. Ref}}$ appears due to the change in the number of up- and down-spin electrons in the spin-flipped excited state:

$$1 - 2M_S^{\text{H.S. Ref}} = (M_S^I(M_S^I + 1) + N_\downarrow^I) - (M^{\text{H.S. Ref}}(M^{\text{H.S. Ref}} + 1) + N_\downarrow^{\text{H.S. Ref}}), \tag{9}$$

$$M_S^I = M^{\text{H.S. Ref}} - 1 \tag{10}$$

$$N_\downarrow^I = N^{\text{H.S. Ref}} + 1. \tag{11}$$

The $\langle\hat{S}^2\rangle_I$ values computed for ethylene under torsion are presented in the main text. Fig. S3 shows the computed $\langle\hat{S}^2\rangle_I$ for the $NV^-$ center, with respect to the number of unoccupied states (and 12 occupied states). The large amount of spin contamination for the $^3A_2$ and $^1A_1$

states is consistent with the finding of Tada et al.[S13] that solids generally have more spin contamination than molecules. The value of $\langle \hat{S}^2 \rangle = 1$ for the $^3E$ state is due to the absence of the $(\bar{v} \downarrow, e_{\{x,y\}} \uparrow)$ states from the set of target states. Such states may be included, in principle, from a multi-reference approach to SF-BSE, analogous to the "mixed reference" approach to SF-TDDFT in Lee et al.[S14].

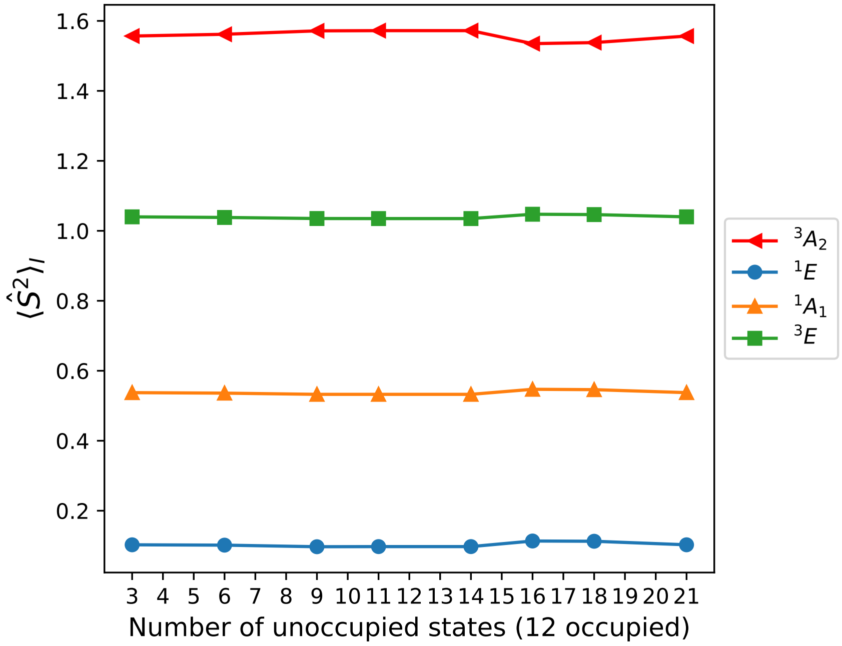


Figure S3: $\langle \hat{S}^2 \rangle_I$ for the $NV^-$ center, with respect to the number of unoccupied states (and 12 occupied states).

# 3 Ethylene potential-energy surfaces from SF-BSE with quasiparticle energies

The single-particle energies that appear in the Bethe-Salpeter Equation are quasiparticle energies. However, as discussed in the main text, we instead use Kohn-Sham eigenvalues. Apart from the usual difficulty of certain single-particle excitations containing spin-multiplet solutions to Dyson's Equation in open-shell systems,[S4] the electronic structure of systems

like triplet ethylene pose additional difficulty for using quasiparticle energies.

With the use of GPP to eliminate the difficulty of multiplets, we can consider the quasiparticle shifts of the Kohn-Sham energies. For singlet ethylene, this proceeds as usual for molecules or solids, with occupied states lowering in energy and unoccupied, rising (Fig. S4a and c). However, triplet ethylene, the high-spin reference state, has its up-spin $\pi$ and $\pi^*$ occupied and down-spin, unoccupied. The Kohn-Sham eigenvalues place the $\pi\downarrow$ energy below the (occupied) $\pi^*\uparrow$ energy. When introducing quasiparticle shifts, the unoccupied down-spin orbitals are raised in energy, above either the occupied up-spin orbitals. Transitions involving flipping an electron in the $\pi^*\uparrow$ orbital to the $\pi\downarrow$ orbital now have a positive energy difference, when including quasiparticle shifts.

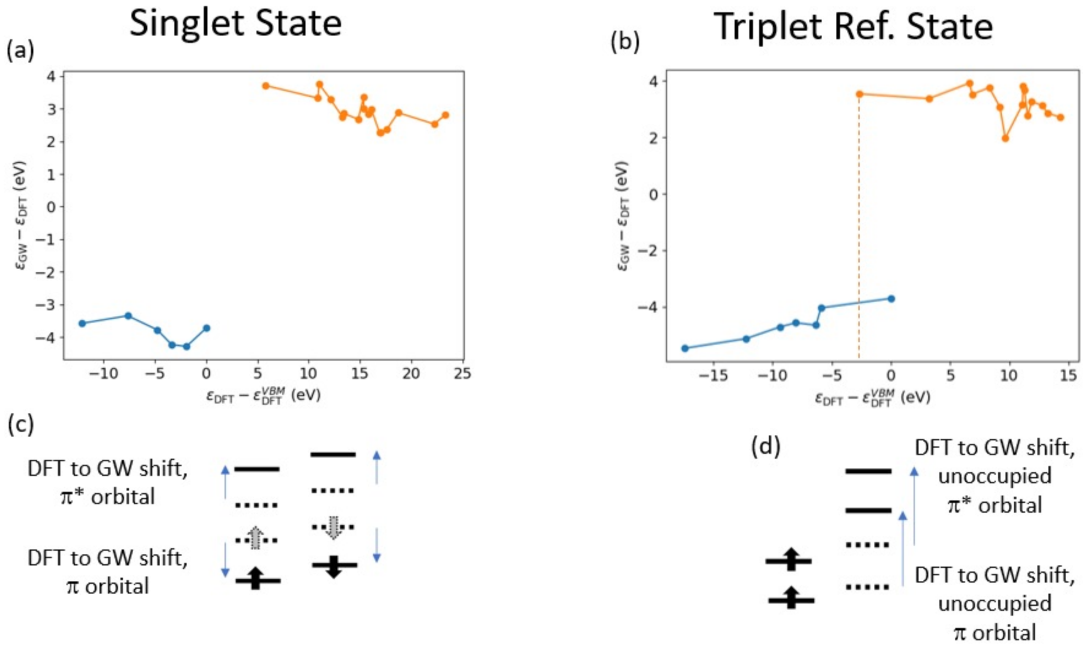


Figure S4: The quasiparticle shifts for ethylene at zero torsion. (a) Quasiparticle shifts for singlet ethylene, (b) quasiparticle shifts for triplet ethylene, the high-spin reference state for SF-BSE, (c) schematic of the quasiparticle shifts for the ethylene frontier orbitals for singlet ethylene, (d) schematic of the quasiparticle shifts for the ethylene frontier orbitals for triplet ethylene. The orange line in (b) is a guide to note that the unoccupied states in triplet ethylene have Kohn-Sham energy eigenvalues below the HOMO.

The energy surfaces for ethylene when using quasiparticle energies in Fig. S5 exhibit some notable disagreements with the energy surfaces computed with Kohn-Sham energies, as in the main text. Notably, the energies for the $N$ state at 10° and 15° torsion are lower in energy than zero torsion by tens of meV. While the zero-torsion transition energies ( N$\rightarrow$ T $= 4.19\ eV$, N$\rightarrow$ V = 8.01 eV) are in good agreement with experiment and our KS-based results, the computed torsion barrier energy 2.93 eV is lower than that of SF-BSE with Kohn-Sham eigenvalues by 32 meV.

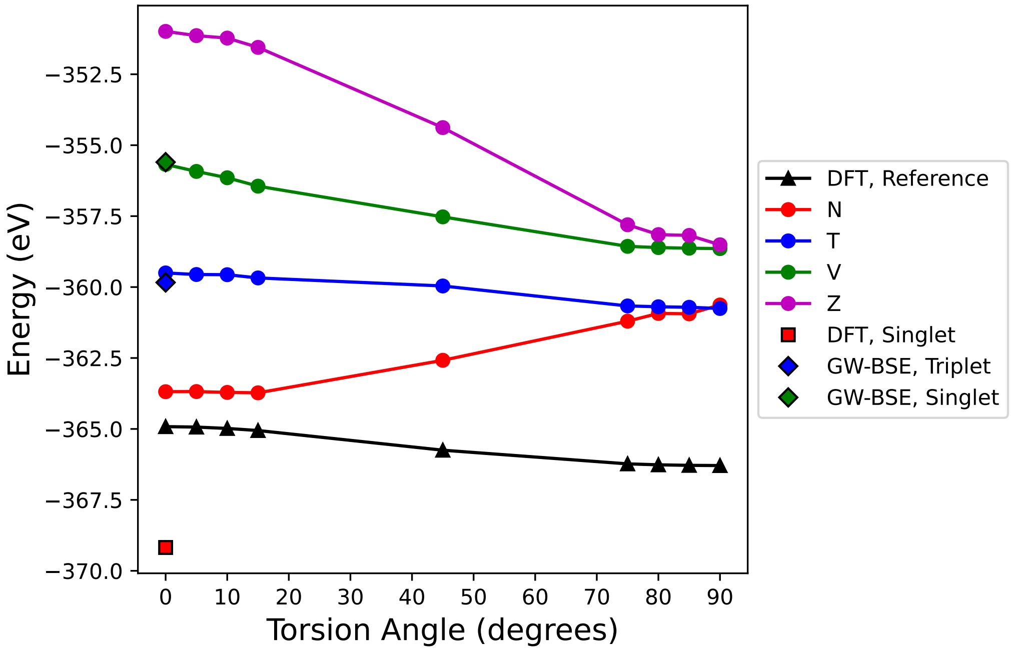


Figure S5: The potential-energy surfaces for ethylene under torsion, computed via SF-BSE with GPP quasiparticle energies.

# 4 Ethylene potential-energy surfaces from SF-BSE with restricted Kohn-Sham

We calculate restricted Kohn-Sham states from Octopus by performing an unpolarized calculation in which occupations are set to 1 for two states, and are 2 or 0 for the others. Then we export a wavefunction file for BerkeleyGW, and manually construct a spin-polarized wave-

function file with identical spin-up and spin-down channels. In the presence of degeneracy at 90°, we split the occupations among pairs of orbitals.

Fig. S6 shows the potential-energy surfaces for the ethylene N, T, V, and Z states, computed via SF-BSE with restricted Kohn-Sham orbitals. The $\pi$ and $\pi^*$ orbitals (with respect to zero torsion) are singly occupied within spin-independent DFT, then spin channels are explicitly introduced by copying the computed Kohn-Sham orbitals to up- and down-spin channels, with the up-spin channel having its frontier orbitals occupied.

There are qualitative differences in the surfaces computed with restricted Kohn-Sham orbitals compared to unrestricted (spin-polarized), as in the main text. The $N$ and $T$ surfaces are no longer monotonic, with a minimum in the $N$ surface appearing around 5°.

The computed values using restricted orbitals agree fairly well with those computed with the usual unrestricted. The torsion barrier is 3.45 eV, within 20 meV of the value presented in the main text. The $N \to T$ transition energy at zero torsion is 3.85 eV, within about 22 meV of the unrestricted result, and within 10 meV to that of conventional $GW$-BSE. The $N \to V$ transition energy at zero torsion is 7.77 eV, within about 20 meV of the unrestricted result, and within about 30 meV to that of conventional $GW$-BSE.

In sum, the use of restricted orbitals for SF-BSE may yield some undesirable features that are not present in the unrestricted case. However, transition energies of interest for both ethylene and the $NV^-$ are in quite good agreement between restricted and unrestricted Kohn-Sham in SF-BSE, and restricted Kohn-Sham has desirable aspects such as less computational expense in generating unoccupied states and definite relations among degenerate orbitals in the spin-up and -down channels. Calculating SF-BSE with restricted Kohn-Sham orbitals may therefore provide a good first pass for challenging systems with large numbers of unpaired spins.

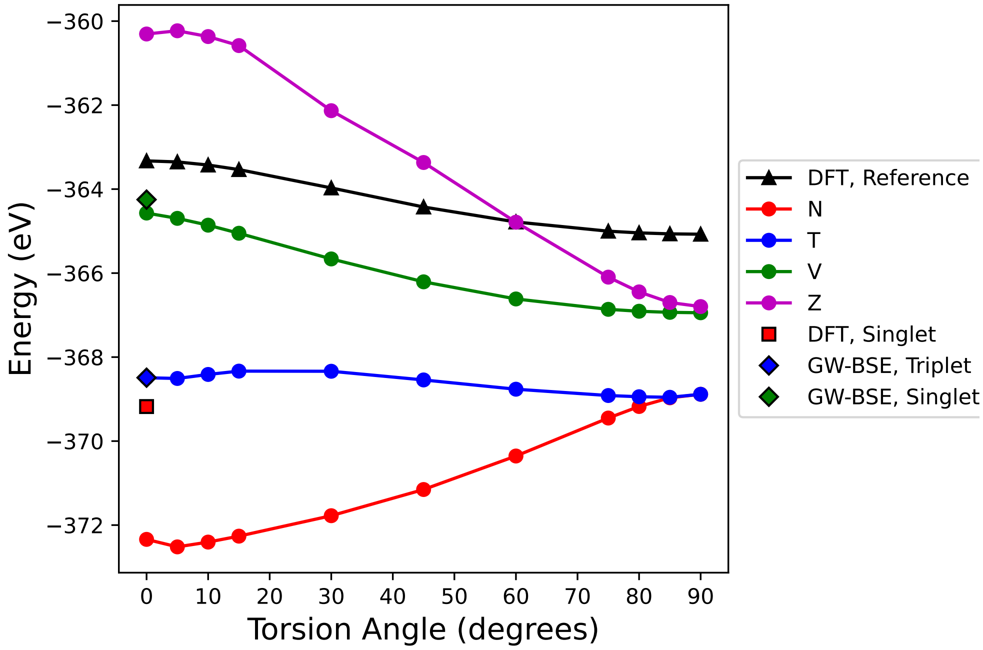


Figure S6: The potential-energy surfaces for ethylene under torsion, computed via SF-BSE with restricted Kohn-Sham orbitals.

# 5 SF-BSE with KS eigenvalues vs. *GW*-BSE for ethylene at zero torsion

To analyze the remarkable agreement for the $N \rightarrow T$ and $N \rightarrow V$ transitions computed in *GW*-BSE and SF-BSE with Kohn-Sham orbital eigenvalues, we investigate the results each method yields with as few electron-hole transitions as possible and note the size of the contributions to the BSE Hamiltonians.

For conventional *GW*-BSE, the minimum size is the transition from the occupied $\pi$ orbital to the unoccupied $\pi^*$ orbital. The quasiparticle energy difference $(D)$ between these orbitals is 12.54 eV. The Direct Kernel $(K^D)$ matrix element is -4.66 eV, and the Exchange Kernel

$(K^X)$ is -2.82 eV. From Eq. 25 in Rohlfing and Louie[S15],

$$H^{GW-\text{BSE}} = \begin{bmatrix} D + K^D + K^X & 0 & 0 & K^X \\ 0 & D + K^D & 0 & 0 \\ 0 & 0 & D + K^D 0 & \\ K^X & 0 & 0 & D + K^D + K^X \end{bmatrix}, \tag{12}$$

with transitions ordered by spin index (now considered explicitly), $(\pi \uparrow, \pi^* \uparrow), (\pi \uparrow, \pi^* \downarrow), (\pi \downarrow, \pi^* \uparrow), (\pi \downarrow, \pi^* \downarrow)$. In our particular case, the matrix elements (in eV) are

$$H^{GW-\text{BSE}} = \begin{bmatrix} 5.06 & 0 & 0 & -2.82 \\ 0 & 7.88 & 0 & \\ 0 & 0 & 7.88 & 0 \\ -2.82 & 0 & 0 & 5.06 \end{bmatrix}, \tag{13}$$

For SF-BSE, the minimal basis set is instead $(\pi^* \uparrow, \pi \downarrow), (\pi \uparrow, \pi \downarrow), (\pi^* \uparrow, \pi^* \downarrow), (\pi \uparrow, \pi^* \downarrow)$, and the four (Kohn-Sham) energy differences are -2.70 eV, 3.22 eV, 3.20 eV, and 9.11 eV. The $K^D$ values are

$$\begin{aligned} K^D_{(\pi^*\uparrow,\pi\downarrow);(\pi^*\uparrow,\pi\downarrow)} &= -2.94 \text{ eV} \\ K^D_{(\pi\uparrow,\pi^*\downarrow);(\pi\uparrow,\pi^*\downarrow)} &= -2.73 \text{ eV} \\ K^D_{(\pi^*\uparrow,\pi^*\downarrow);(\pi^*\uparrow,\pi^*\downarrow)} &= -2.71 \text{ eV} \\ K^D_{(\pi\uparrow,\pi\downarrow);(\pi\uparrow,\pi\downarrow)} &= -3.44 \text{ eV} \\ K^D_{(\pi^*\uparrow,\pi\downarrow);(\pi\uparrow,\pi^*\downarrow)} &= -1.84 \text{ eV} \\ K^D_{(\pi\uparrow,\pi^*\downarrow);(\pi^*\uparrow,\pi\downarrow)} &= -1.84 \text{ eV} \\ K^D_{(\pi\uparrow,\pi\downarrow);(\pi^*\uparrow,\pi^*\downarrow)} &= -1.84 \text{ eV} \\ K^D_{(\pi^*\uparrow,\pi^*\downarrow);(\pi\uparrow,\pi\downarrow)} &= -1.84 \text{ eV}, \end{aligned} \tag{14}$$

with the others zero.

## 6 Energies of SF-BSE excitations in $NV^-$ center

We compare the values for the excitation energies for the in-gap many-body states for the $NV^-$ center in diamond, when using either Kohn-Sham orbital eigenvalues or quasiparticle energies (as estimated with GPP) for the term in the BSE involving energy differences between unoccupied and occupied states. In Table S1, we see that the use of quasiparticle energies amounts to a rigid shift of the excitation energies, of about 0.9 eV for the $^3A_2$, $^1E$, and $^1A_1$ states, and 1.0 eV for $^3E$. Note, however, this rigid shift has little affect on the energy differences between these states.

**Table S1: Excitation energies in eV for in-gap many-body states for the $NV^-$ center in diamond. "KS" refers to using the Kohn-Sham orbital eigenvalues in the SF-BSE Hamiltonian, and "GPP" refers to the use of quasiparticle energies estimated within the generalized plasmon pole approximation.**

| Excitation | Unrestricted, KS | Unrestricted, GPP | Difference |
|---|---|---|---|
| $^3A_2$ | -0.052 | 0.846 | 0.898 |
| $^1E_2$ | 0.385 | 1.290 | 0.906 |
| $^1A_1$ | 0.993 | 1.883 | 0.890 |
| $^3E$ | 2.013 | 3.056 | 1.043 |

To better understand this relatively constant difference for the in-gap many-body states, we consider a model in which the quasiparticle shift in energy is a linear fit to the Kohn-Sham eigenvalues: $\epsilon_n^{\mathrm{QP}} = (1+m)\epsilon_n^{\mathrm{KS}} + b$, for some slope $m$ and $b$, which will generally have different values for occupied ($m_v$,$b_v$) and unoccupied states ($m_c$,$b_c$). In the BSE, we have

$$\left(\epsilon_c^{\mathrm{QP}} - \epsilon_v^{\mathrm{QP}}\right) A_{vc}^I \delta_{vv'} \delta_{cc'} + K_{vc,v'c'} A_{v'c'}^I = \Omega^I A_{vc}^I \tag{15}$$

$$\left((1+m_c)\epsilon_c^{\mathrm{KS}} + b_c - (1+m_v)\epsilon_v^{\mathrm{KS}} + b_v)\right) A_{vc}^I \delta_{vv'} \delta_{cc'} + K_{vc,v'c'} A_{v'c'}^I = \Omega^I A_{vc}^I$$

.

The quasiparticle shifts for the $NV^-$ displayed in Fig. S7 shows nearly the same slope for the lines of best fit for the occupied states ($m_v = 0.14$) and for the unoccupied states ($m_c = 0.16$). The lines are offset by about 0.9 eV, or $\Delta = b_c - b_v = 0.9$ eV. We can then approximate the BSE as

$$(1+m)\left(\epsilon_c^{\mathrm{KS}} - \epsilon_v^{\mathrm{KS}}\right) A_{vc}^I \delta_{vv'}\delta_{cc'} + K_{vc,v'c'} A_{v'c'}^I = (\Omega^I - \Delta) A_{vc}^I. \tag{16}$$

The SF-BSE excitation energies computed with the Kohn-Sham eigenvalues can be used to approximate the excitation energies computed with the quasiparticle energies by adding to them the quasiparticle shift of the HOMO and LUMO, and then scaling the KS eigenvalue energy differences by $1+m$, provided the quasiparticle shifts have approximately the same slope.

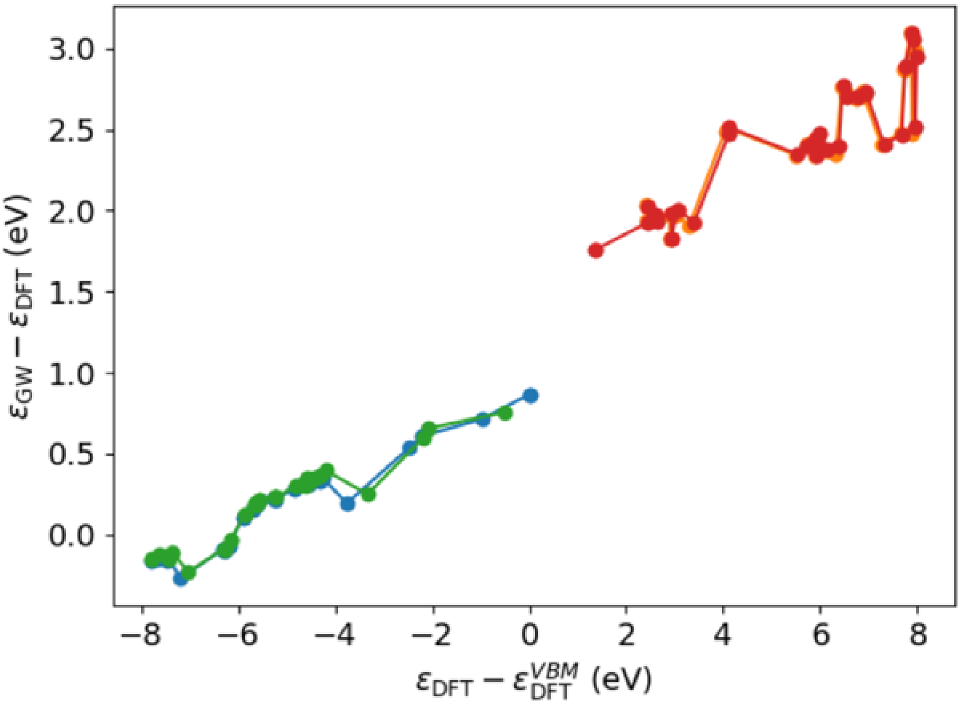


Figure S7: Quasiparticle shifts for $NV^-$. Blue and green: quasiparticle shifts for occupied spin up and down states, respectively. Red and orange: quasiparticle shifts for unoccupied spin up and down states, respectively.

The DFT bandstructure in Fig. S8 for the 2×2×2 supercell for the $NV^-$ center defect

shows relatively high dispersion for the in-gap defect states, which indicates spurious interactions between periodic images of the defect. While the 2×2×2 supercell appears to be too small to compute a physical bandstructure, Table S2 shows good agreement between the quasiparticle energies with this 64-atom supercell and those of Ma et al.[S16] which uses a 256-atom supercell.

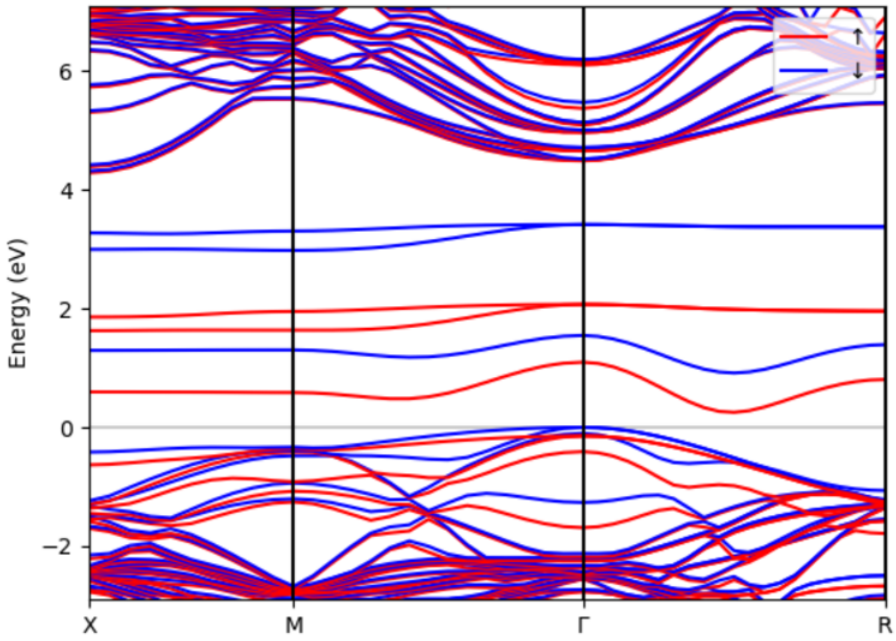


Figure S8: The bandstructure of the 2×2×2 diamond supercell for the $NV^-$ center defect. The dispersion of the in-gap states indicates interactions between periodic images of the defect.

**Table S2: Quasiparticle energy differences, in eV, computed with one-shot $G_0W_0$ and the Generalized Plasmon Pole model for the self-energy operator frequency dependence.**

| | Present | Ma et al.[S16] |
|---|---|---|
| $E(\bar{v},\beta) - E(v,\alpha)$ | 0.5 | 0.6 |
| $E(\{e_x, e_y\},\alpha) - E(v,\alpha)$ | 1.1 | 1.2 |
| $E(\{\bar{e}_x, \bar{e}_y\},\beta) - E(v,\alpha)$ | 3.4 | 3.3 |

# 7 Convergence of Ethylene Torsion Potential with respect to number of transitions

In Fig. S9 we demonstrate the convergence of the ethylene torsion barrier with respect to the number of unoccupied states included in the SF-BSE basis set of transitions, up to 100 unoccupied states. With 55 unoccupied orbitals, the value of the torsion potential is in agreement within a few meV with respect to the value with 100 unoccupied orbitals.

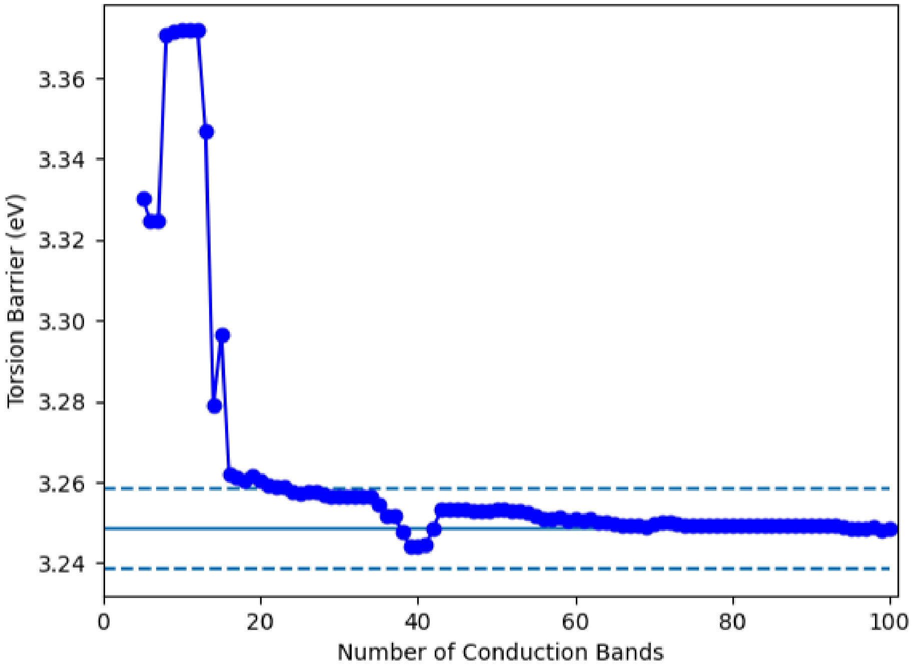


Figure S9: Convergence of the ethylene torsion barrier with respect to the number of unoccupied states included in the SF-BSE basis set of transitions. The number of occupied states is fixed at five.

To gain insight into the behavior of this convergence, we investigated the partial density of states (PDOS) of the H and C valence states for ethylene under zero torsion in Fig. S10 and 90° torsion in Fig. S11. Unoccupied (down-spin) orbital 55 has an energy of about 35 eV, and the PDOS shows that beyond this energy the atomic-like states no longer provide significant contributions to the unoccupied states. This indicates convergence of the eigenvalues of the SF-BSE Hamiltonian is achieved when all localized states are included in the basis set.

Fig. S12 shows the convergence of the ethylene torsion barrier with respect to the number

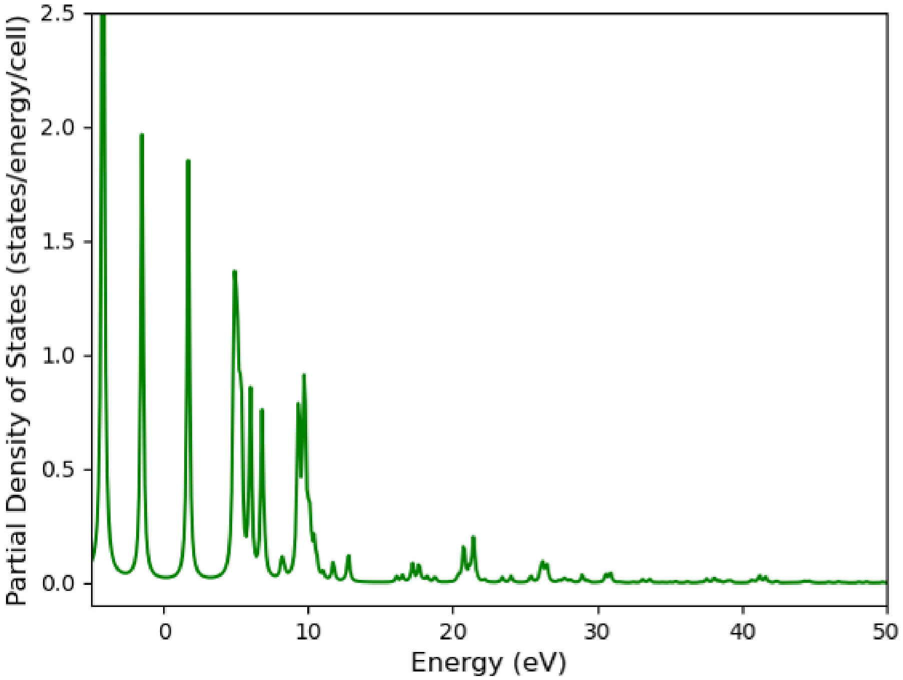


Figure S10: Partial density of states for ethylene at 0° torsion summed over all C $2s2p$ and H $1s$ states.

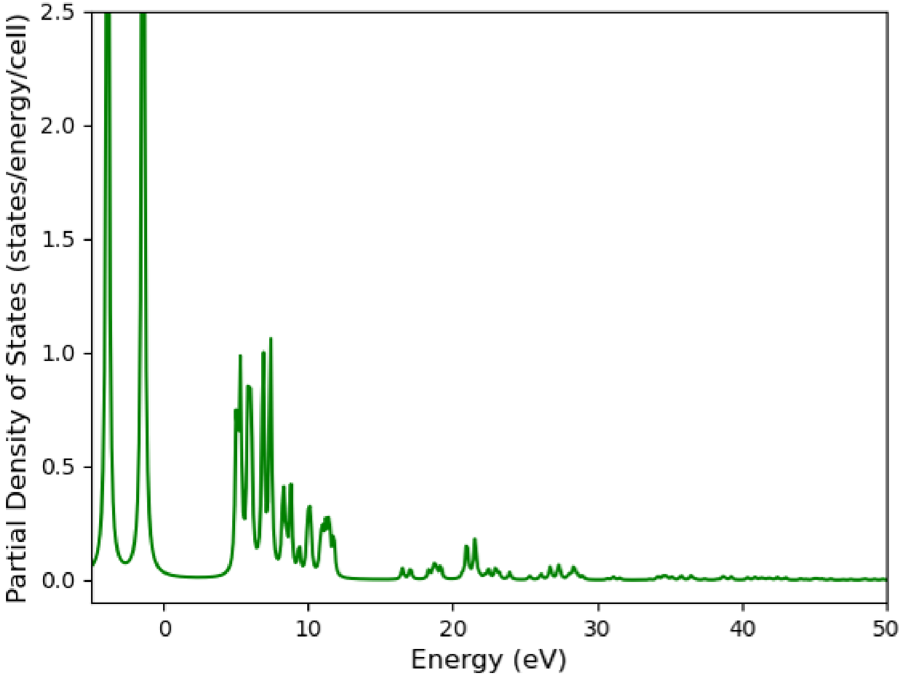


Figure S11: Partial density of states for ethylene at 90° torsion summed over all C $2s2p$ and H $1s$ states.

of occupied states. The value continues to lower with increasing number of occupied orbitals.

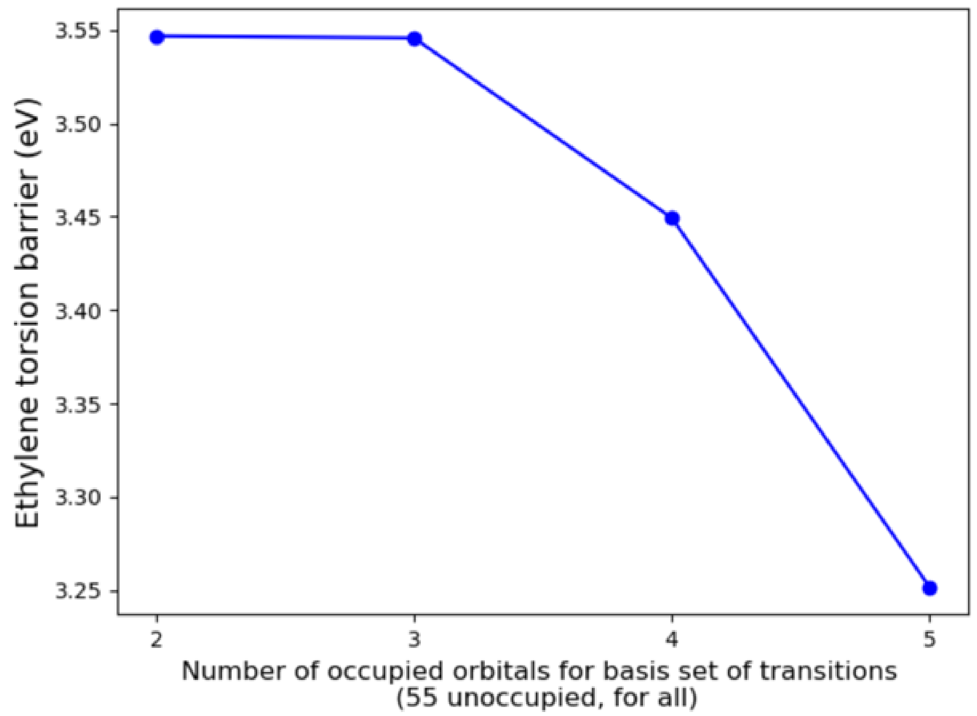


Figure S12: Convergence of the ethylene torsion barrier with respect to the number of occupied states included in the SF-BSE basis set of transitions. The maximum number of occupied states is 5.

# 8 Convergence of transition energies in $NV^-$

Figs. S13 and S14 show the convergence of the transition energies for $NV^-$ with respect to the number of occupied and unoccupied bands, respectively. We expect that the use of 12 occupied and 11 unoccupied bands gives converged transition energies within tens of meV.

# 9 The Kohn-Sham energy eigenvalues of the frontier orbitals of ethylene under torsion

Fig. S15 compares the Kohn-Sham orbital energy eigenvalues for the ethylene $\pi$ and $\pi^*$ frontier orbitals (labelled by their symmetry for zero torsion), as a function of torsion angle,

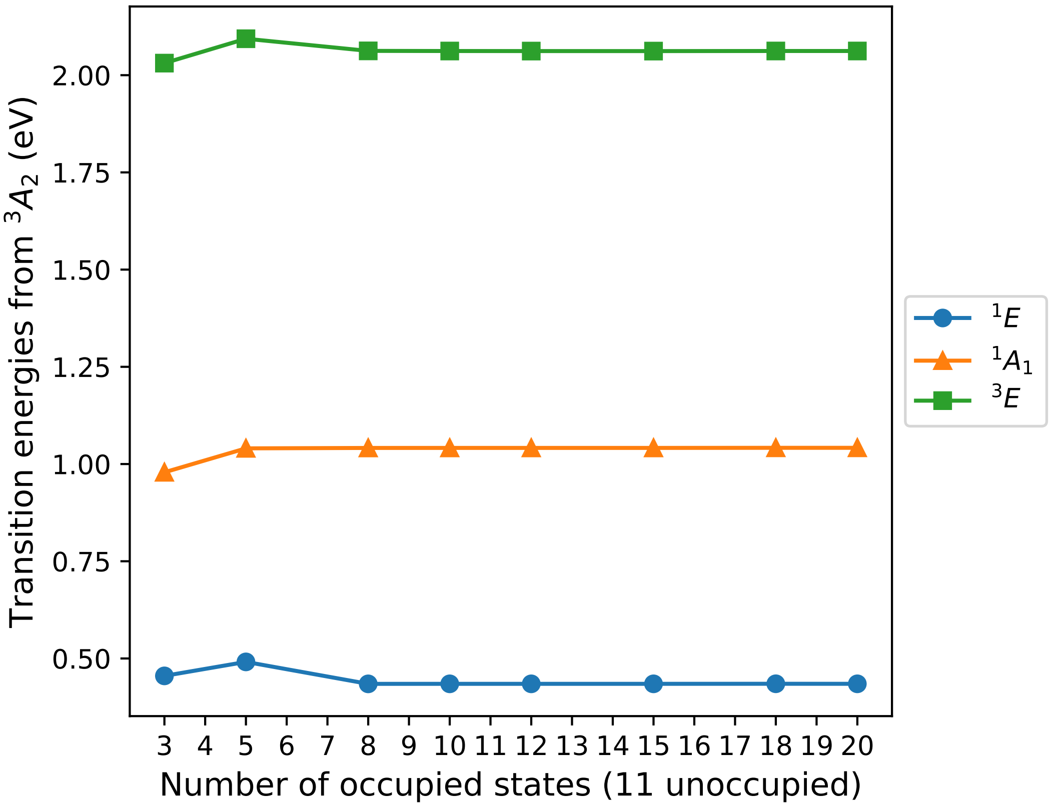


Figure S13: Convergence of transition energies in $NV^-$ with respect to the number of occupied orbitals, with 11 unoccupied orbitals.

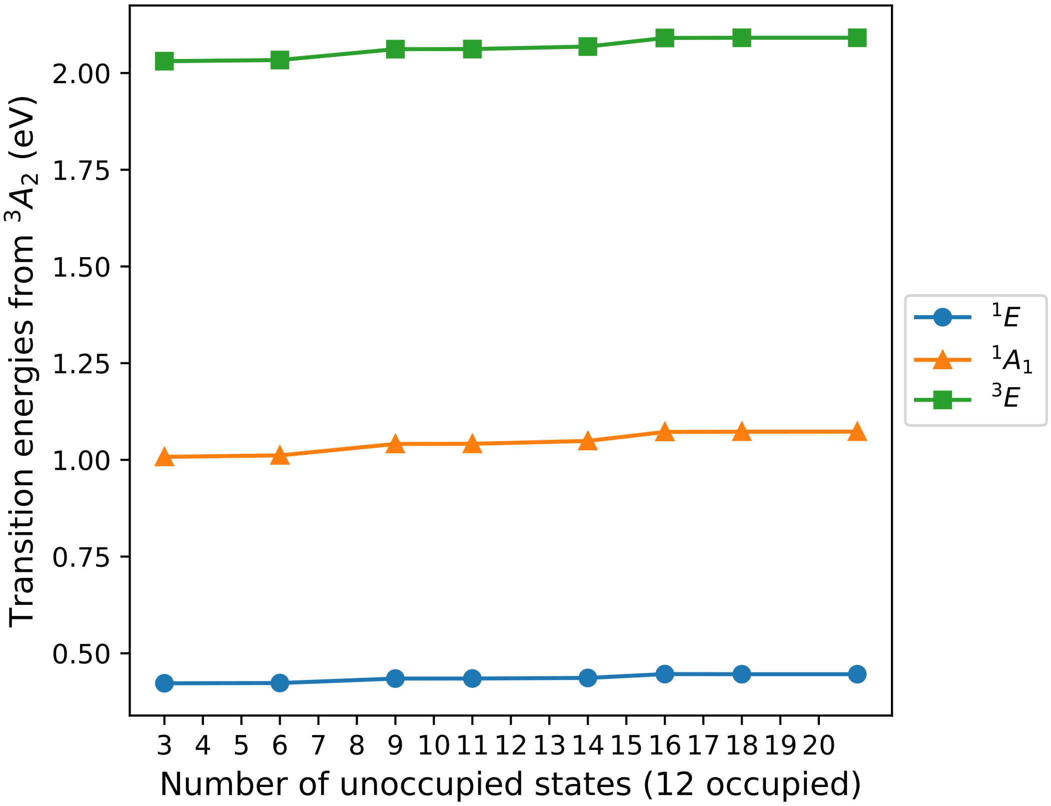


Figure S14: Convergence of transition energies in $NV^-$ with respect to the number of unoccupied orbitals, with 12 unoccupied orbitals.

for triplet and singlet spin symmetries. The triplet spin symmetry, used for the high-spin reference state for SF-BSE, shows a difference of about 3.2 eV for the energies of both the $\pi$ and $\pi^*$ orbitals between the up- and down-spin channels, at zero torsion. The singlet spin symmetry ("unpolarized") orbital eigenvalues are, within 100 meV, the average of the spin-polarized eigenvalues. At higher torsion angles, the unpolarized eigenvalues are 0.9 eV higher than the spin-up eigenvalues and 1.6 eV below the spin-down eigenvalues.

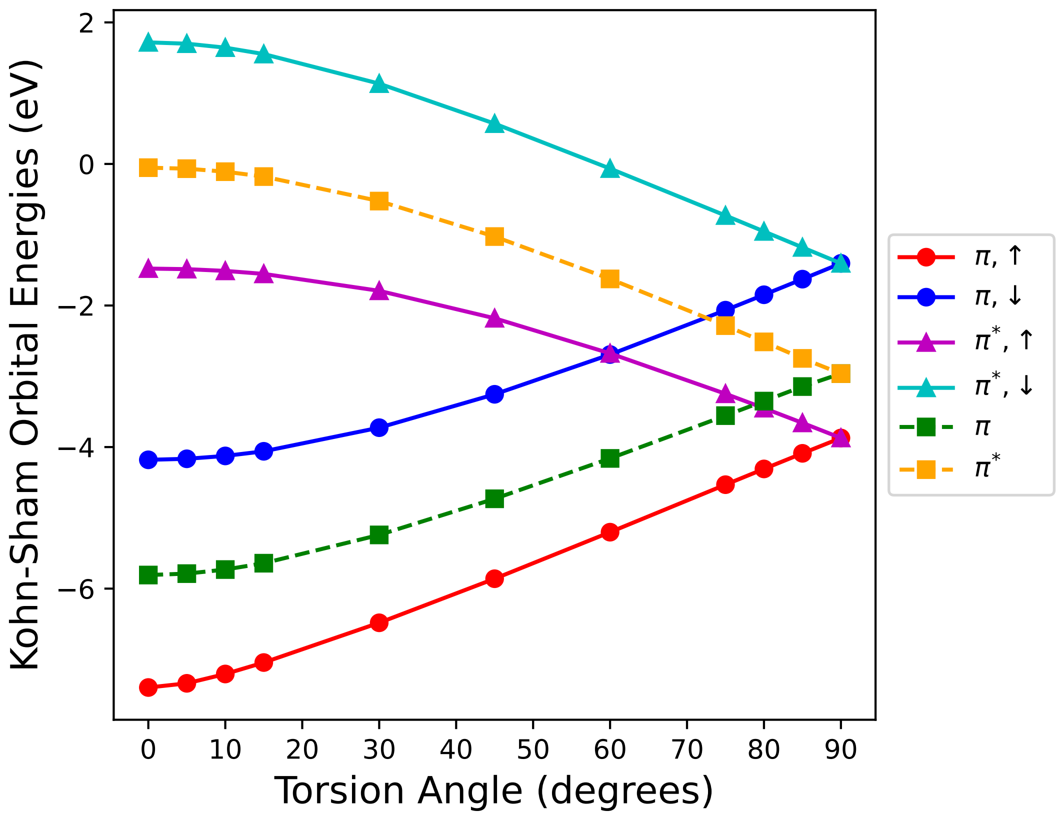


Figure S15: Kohn-Sham orbital energies of ethylene as a function of torsion angle, comparing the $\pi$ and $\pi^*$ of the spin-polarized high-spin reference $(\uparrow, \downarrow)$ with those the unpolarized closed shell calculation.

# 10 Ethylene transition energies within conventional $GW$-BSE, and convergence of SF-BSE transition energies with this box size

The convergence parameters for the calculation of transition energies from ethylene under 0° of torsion from conventional $GW$-BSE differ from that of the results from SF-BSE. To achieve results comparable to experiment with $GW$-BSE, the box size is 10.84 Å × 9.30 Å × 8.54 Å, larger than the box size that is double that which contains 99% of the charge density (the standard heuristic for using Coulomb truncation schemes in BerkeleyGW[S17]). The BSE Kernel is calculated with 6 valence states and 500 conduction states. Otherwise, calculation parameters are the same as with SF-BSE.

**Table S3: Ethylene transition energies from a conventional $GW$-BSE calculation with a box size of 10.84 Å × 9.30 Å × 8.54 Å**

| Transition energies (eV) | QP, with K | QP, no K | KS, with K | KS, no K |
|---|---|---|---|---|
| $N \to T$ | 8.09 | 12.55 | 1.27 | 5.57 |
| $N \to V$ | 3.85 | 12.55 | -3.00 | 5.57 |

**Table S4: Ethylene transition energies computed within SF-BSE with a box size of 10.84 Å × 9.30 Å × 8.54 Å, with respect to number of empty states in the Chi summation.**

| Transition energies (eV) | 860 | 2090 | 3000 |
|---|---|---|---|
| $N \to T$ | 4.52 | 4.05 | 4.04 |
| $N \to V$ | 6.80 | 7.54 | 7.53 |

With the larger box size of 10.84 Å × 9.30 Å × 8.54 Å, as used for the conventional $GW$-BSE calculations, converged results are only achieved with 2090 empty states (Table S4). With the smaller box size and 860 empty states (as in the main text), the transition energies are 4.07 eV for $N \to T$, 7.95 eV for $N \to V$ which are in good agreement.

# 11 Disregarding BSE Kernel

As shown in Fig. S16, without the BSE kernel, results are both qualitatively and quantitatively different from the correct energy levels, demonstrating the correct physics and splitting captured by the kernel in SF-BSE. Indeed, for the NV$^-$ center, the $^3A_2$, $^1E$, and $^1A_1$ excitations are indistinguishable without including the BSE kernel.

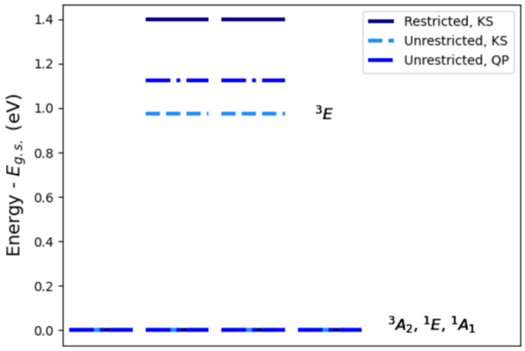


Figure S16: The in-gap many-body defect states, without including the BSE kernel. The states composed of single-particle transitions from $e$ to $e$ are all degenerate.

For ethylene, neglecting the BSE kernel produces qualitatively and quantitatively incorrect results. Most noticeably, all four potential-energy surfaces become degenerate at 90 degrees, in Fig. S17.

# 12 Atomic coordinates of ethylene, Cartesian, Å

```
C   0.67596    0.0       0.0
C  -0.67596    0.0       0.0
H  -1.248847   0.938124  0.0
H  -1.248847  -0.938124  0.0
H   1.248847   0.938124  0.0
H   1.248847  -0.938124  0.0
```

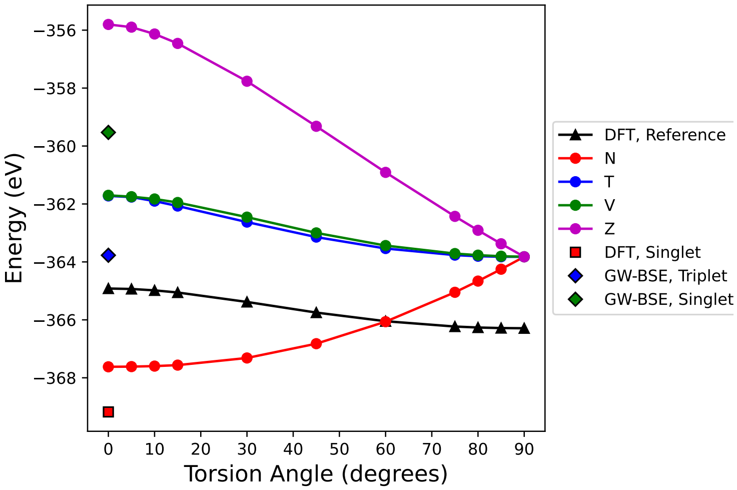


Figure S17: The potential-energy surfaces for ethylene under torsion, neglecting the BSE kernel.

## 13 Atomic coordinates of $NV^-$ center, Cartesian, Å

```
Lattice Vectors:
a_1 =  7.290611999        0.000000000        0.000000000
a_2 =  0.000000000        7.290611999        0.000000000
a_3 =  0.000000000        0.000000000        7.290611999

C          -0.0646803134      -0.0646803134      -0.0646803134
C           0.8460886954       0.8460886954       0.8460886954
C          -0.0676786733       1.7574888720       1.7574888720
C           0.8465567934       2.6675357855       2.6675357855
C           1.7574888720      -0.0676786733       1.7574888720
C           2.6675357855       0.8465567934       2.6675357855
C           1.7574888720       1.7574888720      -0.0676786733
C           2.6675357855       2.6675357855       0.8465567934
C           3.5797580003      -0.0663773464      -0.0663773464
C           4.4827342533       0.8382337835       0.8382337835
C           3.5848692106       1.7590129542       1.7590129542
C           4.5287392958       2.6035572547       2.6035572547
C           5.3992699733      -0.0730590533       1.7653216651
C           6.3148273542       0.8409524453       2.6733094130
C           5.3992699733       1.7653216651      -0.0730590533
C           6.3148273542       2.6733094130       0.8409524453
C          -0.0663773464       3.5797580003      -0.0663773464
C           0.8382337835       4.4827342533       0.8382337835
C          -0.0730590533       5.3992699733       1.7653216651
C           0.8409524453       6.3148273542       2.6733094130
C           1.7590129542       3.5848692106       1.7590129542
C           2.6035572547       4.5287392958       2.6035572547
C           1.7653216651       5.3992699733      -0.0730590533
C           2.6733094130       6.3148273542       0.8409524453
C          -0.0663773464      -0.0663773464       3.5797580003
C           0.8382337835       0.8382337835       4.4827342533
C          -0.0730590533       1.7653216651       5.3992699733
C           0.8409524453       6.3148273542       2.6733094130
C           1.7590129542       3.5848692106       1.7590129542
C           2.6035572547       4.5287392958       2.6035572547
C           1.7653216651       5.3992699733      -0.0730590533
C           2.6733094130       6.3148273542       0.8409524453
C          -0.0663773464      -0.0663773464       3.5797580003
C           0.8382337835       0.8382337835       4.4827342533
```

| | | | |
|---|---|---|---|
| C | -0.0730590533 | 1.7653216651 | 5.3992699733 |
| C | 0.8409524453 | 2.6733094130 | 6.3148273542 |
| C | 1.7653216651 | -0.0730590533 | 5.3992699733 |
| C | 2.6733094130 | 0.8409524453 | 6.3148273542 |
| C | 1.7590129542 | 1.7590129542 | 3.5848692106 |
| C | 2.6035572547 | 2.6035572547 | 4.5287392958 |
| C | -0.0667545877 | 3.5782498797 | 3.5782498797 |
| C | 0.8540126984 | 4.4865445397 | 4.4865445397 |
| C | -0.0557553788 | 5.4026546283 | 5.4026546283 |
| C | 0.8526636511 | 6.3120407451 | 6.3120407451 |
| C | 1.7708249457 | 3.5672802066 | 5.3820988510 |
| C | 2.6856093849 | 4.4803538081 | 6.2958926916 |
| C | 1.7708249457 | 5.3820988510 | 3.5672802066 |
| C | 2.6856093849 | 6.2958926916 | 4.4803538081 |
| C | 3.5782498797 | -0.0667545877 | 3.5782498797 |
| C | 4.4865445397 | 0.8540126984 | 4.4865445397 |
| C | 3.5672802066 | 1.7708249457 | 5.3820988510 |
| C | 4.4803538081 | 2.6856093849 | 6.2958926916 |
| C | 5.4026546283 | -0.0557553788 | 5.4026546283 |
| C | 6.3120407451 | 0.8526636511 | 6.3120407451 |
| C | 5.3820988510 | 1.7708249457 | 3.5672802066 |
| C | 6.2958926916 | 2.6856093849 | 4.4803538081 |
| C | 6.2958926916 | 2.6856093849 | 4.4803538081 |
| C | 3.5782498797 | 3.5782498797 | -0.0667545877 |
| C | 4.4865445397 | 4.4865445397 | 0.8540126984 |
| C | 3.5672802066 | 5.3820988510 | 1.7708249457 |
| C | 4.4803538081 | 6.2958926916 | 2.6856093849 |
| C | 5.3820988510 | 3.5672802066 | 1.7708249457 |
| C | 6.2958926916 | 4.4803538081 | 2.6856093849 |
| C | 5.4026546283 | 5.4026546283 | -0.0557553788 |
| C | 6.3120407451 | 6.3120407451 | 0.8526636511 |
| N | 4.5809280033 | 4.5809280033 | 4.5809280033 |
| C | 3.6266550932 | 5.3982139985 | 5.3982139985 |
| C | 4.4936340966 | 6.3242778007 | 6.3242778007 |
| C | 5.3982139985 | 3.6266550932 | 5.3982139985 |
| C | 6.3242778007 | 4.4936340966 | 6.3242778007 |
| C | 5.3982139985 | 5.3982139985 | 3.6266550932 |
| C | 6.3242778007 | 6.3242778007 | 4.4936340966 |

# References


(S1) Hamann, D. R. Optimized norm-conserving Vanderbilt pseudopotentials. *Phys. Rev. B* **2013**, *88*, 085117.

(S2) Van Setten, M. J.; Giantomassi, M.; Bousquet, E.; Verstraete, M. J.; Hamann, D. R.; Gonze, X.; Rignanese, G.-M. The PseudoDojo: Training and grading a 85 element optimized norm-conserving pseudopotential table. *Comput. Phys. Comm.* **2018**, *226*, 39–54.

(S3) van Setten, M. J.; Caruso, F.; Sharifzadeh, S.; Ren, X.; Scheffler, M.; Liu, F.; Lischner, J.; Lin, L.; Deslippe, J. R.; Louie, S. G.; Yang, C.; Weigend, F.; Neaton, J. B.; Evers, F.; Rinke, P. $GW$100: Benchmarking $G_0W_0$ for molecular systems. *J. Chem. Theory Comput.* **2015**, *11*, 5665–5687.

(S4) Lischner, J.; Deslippe, J.; Jain, M.; Louie, S. G. First-principles calculations of quasiparticle excitations of open-shell condensed matter systems. *Phys. Rev. Lett.* **2012**, *109*, 036406.

(S5) Löwdin, P.-O. Quantum theory of many-particle systems. I. Physical interpretations by means of density matrices, natural spin-orbitals, and convergence problems in the method of configurational interaction. *Phys. Rev.* **1955**, *97*, 1474.

(S6) Li, Z.; Liu, W.; Zhang, Y.; Suo, B. Spin-adapted open-shell time-dependent density functional theory. II. Theory and pilot application. *J. Chem. Phys.* **2011**, *134*, 134101.

(S7) Xu, X.; Yang, K. R.; Truhlar, D. G. Testing noncollinear spin-flip, collinear spin-flip, and conventional time-dependent density functional theory for predicting electronic excitation energies of closed-shell atoms. *J. Chem. Theory Comput.* **2014**, *10*, 2070–2084.

(S8) Monino, E.; Loos, P.-F. Spin-Conserved and Spin-Flip Optical Excitations from the Bethe–Salpeter Equation Formalism. *J. Chem. Theory Comput.* **2021**, *17*, 2852–2867.

(S9) Strinati, G. Application of the Green's functions method to the study of the optical properties of semiconductors. *Riv. Nuovo Cimento* **1988**, *11*, 1.

(S10) Ipatov, A.; Cordova, F.; Doriol, L. J.; Casida, M. E. Excited-state spin-contamination in time-dependent density-functional theory for molecules with open-shell ground states. *J. Mol. Struct.: THEOCHEM* **2009**, *914*, 60–73.

(S11) Zitko, R. SNEG – Mathematica package for symbolic calculations with second-quantization-operator expressions. *Comput. Phys. Commun.* **2011**, *182*, 2259–2264.

(S12) Wang, J.; Becke, A. D.; Smith Jr, V. H. Evaluation of $\langle S^2 \rangle$ in restricted, unrestricted Hartree–Fock, and density functional based theories. *J. Chem. Phys.* **1995**, *102*, 3477–3480.

(S13) Tada, K.; Yamanaka, S.; Kawakami, T.; Kitagawa, Y.; Okumura, M.; Yamaguchi, K.; Tanaka, S. Estimation of spin contamination errors in DFT/plane-wave calculations of solid materials using approximate spin projection scheme. *Chem. Phys. Lett.* **2021**, *765*, 138291.

(S14) Lee, S.; Filatov, M.; Lee, S.; Choi, C. H. Eliminating spin-contamination of spin-flip time dependent density functional theory within linear response formalism by the use of zeroth-order mixed-reference (MR) reduced density matrix. *J. Chem. Phys.* **2018**, *149*, 104101.

(S15) Rohlfing, M.; Louie, S. G. Electron-hole excitations and optical spectra from first principles. *Phys. Rev. B* **2000**, *62*, 4927–4944.

(S16) Ma, Y.; Rohlfing, M.; Gali, A. Excited states of the negatively charged nitrogen-vacancy color center in diamond. *Phys. Rev. B* **2010**, *81*, 041204(R).

(S17) Deslippe, J.; Samsonidze, G.; Strubbe, D. A.; Jain, M.; Cohen, M. L.; Louie, S. G. BerkeleyGW: A massively parallel computer package for the calculation of the quasi-particle and optical properties of materials and nanostructures. *Comput. Phys. Commun.* **2012**, *183*, 1269–1289.
